# Supplementary material for: Lagrangian Particle Classification and Lagrangian Flux Identities for a Moving Hypersurface
Source: arXiv:2506.04125 source file (2025-06-04)
Supplement: Supplementary file 1 [file appendix.tex]

\section{Appendix}
\label{sec:appendix}

\subsection{The proof of theorem \ref{thm:div}}
\label{sec:pf_GDT}

\begin{proof}
We can't apply the divergence theorem to $\mathcal{S}$ directly, 
since $\mathcal{S}$ may be self-intersecting. 
We prove this theorem in two strategic steps. 
Firstly, we will pull back the integral over $\mathcal{D}^{n}$ 
to the integral over  $D^{m}$. 
Secondly, we will apply the classical divergence theorem. 
By the area formula \eqref{eq:AreaFormula}, we have 
\begin{equation}
  \label{eq:Original}
 \sum\limits_{n}^{}n\int_{\mathcal{D}^{n}}\nabla\cdot\mathbf{A}
 \dif\mathbf{x}=\int\limits_{D^{m}}^{}
 \nabla\cdot\mathbf{A}(\varphi (\mathbf{p})) J_\varphi
  \mathrm{d}\mathbf{p},
\end{equation}
where $\mathbf{x}=\varphi(\mathbf{p})$ and 
$J_{\varphi}$ is the Jacobian determinant of $\varphi$, 
$\mathbf{A}=(A_{1},\ldots,A_{m})$ and $\mathbf{p}=(p_{1},\ldots,p_{m})$. 
By the chain rule of derivative, 
we have $\frac{\partial A_{i}}{\partial p_j}
=\sum\limits_{k=1}^{n}\frac{\partial A_i}{\partial x_k}
\frac{\partial \varphi_k}{\partial p_j}$, 
$i,j=1,\ldots,m$. $\frac{\partial A_j}{\partial x_j}$ 
can be solved from this system of equations by Cramer's Rule, that is
\begin{equation}
\label{eq:DetM}
  \frac{\partial A_j}{\partial x_j}=\frac{\det
    \begin{bmatrix}
      \pdfFrac{\varphi_{1}}{p_{1}}&\cdots&
      \pdfFrac{\varphi_{j-1}}{p_{1}}&\pdfFrac{A_{j}}{p_{1}}&
      \pdfFrac{\varphi_{j+1}}{p_{1}}&\cdots&
      \pdfFrac{\varphi_{m}}{p_{1}}\\
      \vdots&\ddots&\vdots&\vdots&\vdots&\ddots&\vdots\\
      \pdfFrac{\varphi_{1}}{p_{m}}&\cdots&
      \pdfFrac{\varphi_{j-1}}{p_{m}}&\pdfFrac{A_{j}}{p_{m}}&
      \pdfFrac{\varphi_{j+1}}{p_{m}}&\cdots&
      \pdfFrac{\varphi_{m}}{p_{m}}
    \end{bmatrix}
}{J_{\varphi}}:=\frac{\det(M_{j})}{J_\varphi}.
\end{equation}

We want to rewrite $\det (M_{j})$ as 
the divergence of some vector fields. 
Mark $M_{i,j}$ as the cofactor of matrix $\dif\varphi$ on $(i,j)$, 
we have 
\begin{equation}
\label{eq:DetM0}
  \begin{aligned}
    \det (M_{j})&=\sum\limits_{i=1}^{m}(-1)^{i+j}
    \frac{\partial A_j}{\partial p_i}M_{i,j}\\
&=\sum\limits_{i=1}^{m}(-1)^{i+j}
\left[\frac{\partial}{\partial p_{i}}\left(A_{j}M_{i,j}\right)
-A_j\frac{\partial M_{i,j}}{\partial p_i}\right]\\
&=\sum\limits_{i=1}^{m} \frac{\partial}{\partial p_{i}}
((-1)^{i+j}A_{j}M_{i,j})-A_{j}
\sum\limits_{i=1}^{m}(-1)^{i+j}
\frac{\partial M_{i,j}}{\partial p_i},
  \end{aligned}
\end{equation}
where the first step is due to Laplace's formula, 
the second step is due to 
$\frac{\partial}{\partial p_{i}}(A_{j} M_{i,j})
=A_j\frac{\partial M_{i,j}}{\partial p_i}
+\frac{\partial A_j}{\partial p_i}M_{i,j}$.

On the other hand, we have 
\begin{equation}
\label{eq:DetM1}
\begin{aligned}
  &\sum\limits_{i=1}^{m}(-1)^{i+j}\frac{\partial M_{i,j}}{\partial p_i}\\
  =&\det\begin{bmatrix}
  \pdfFrac{\varphi_{1}}{p_{1}}&\cdots&
  \pdfFrac{\varphi_{j-1}}{p_{1}}&\pdfFrac{}{p_{1}}&
  \pdfFrac{\varphi_{j+1}}{p_{1}}&\cdots&
  \pdfFrac{\varphi_{m}}{p_{1}}\\
  \vdots&\ddots&\vdots&\vdots&\vdots&\ddots&\vdots\\
  \pdfFrac{\varphi_{1}}{p_{m}}&\cdots&\pdfFrac{\varphi_{j-1}}{p_{m}}&
  \pdfFrac{}{p_{m}}&\pdfFrac{\varphi_{j+1}}{p_{m}}&\cdots&
  \pdfFrac{\varphi_{m}}{p_{m}}
  \end{bmatrix}
\\
=&\sum\limits_{(i_1,\ldots,i_m)\in S_{m}}^{}e_{i_1,\ldots,i_m}
\frac{\partial}{\partial p_{i_{j}}}
\left(\frac{\partial \varphi_1}{\partial p_{i_{1}}}
\ldots\pdfFrac{\varphi_{j-1}}{p_{i_{j-1}}}
\pdfFrac{\varphi_{j+1}}{p_{i_{j+1}}}\ldots\frac{\partial
  \varphi_m}{\partial p_{i_{m}}}\right)\\
=&\sum\limits_{(i_1,\ldots,i_m)\in S_{m}}^{}
e_{i_1,\ldots,i_m}\sum\limits_{k=1,k\neq j}^{m}
\frac{\partial^{2} \varphi_{k}}{\partial p_{i_{k}}\partial p_{i_{j}}}
\left(\frac{\partial \varphi_1}{\partial p_{i_{1}}}\ldots
\frac{\partial\hat{\varphi}_j}{\partial \hat{p}_{i_{j}}}
\ldots\pdfFrac{\hat{\varphi}_{k}}{\hat{p}_{i_{k}}}\ldots
\frac{\partial\varphi_m}{\partial p_{i_{m}}}\right)\\
=&0,
  \end{aligned}
\end{equation}
$\hat{\varphi}_{j}$ means we omit this element. 
The second step is from the definition of determinant, $S_{m}$ 
is the permutation group with order m, and $e_{i_1,i_2,\ldots,i_m}$ 
is Levi-Civita symbol which is anti-symmetric. 
In the last step, 
$\frac{\partial^{2} \varphi_{k}}{\partial p_{i_{j}}\partial p_{i_{k}}}$
 is symmetric and $e_{i_1,i_2,\ldots,i_m}$ is anti-symmetric, 
so the whole summation is zero. 
Now the integral becomes
\begin{equation}
  \label{eq:GDT_Equiv_form_1}
  \begin{aligned}
I&=\int\limits_{D^{m}}^{} \nabla\cdot\mathbf{A}(\varphi (\mathbf{p}))
J_\varphi \mathrm{d}\mathbf{p}\\
&=\int\limits_{D^{m}}\sum_{j=1}^{m}\sum_{i=1}^{m}\pdfFrac{}{p_{i}}
\left((-1)^{i+j}A_{j}(\varphi(\mathbf{p}))M_{i,j}\right)
\mathrm{d}\mathbf{p}.\\ 
  \end{aligned}
\end{equation}
where the first step is from equation \eqref{eq:DetM}, the second
step is from equation \eqref{eq:DetM0} and \eqref{eq:DetM1}.

Set 
\begin{equation}
  \label{eq:aux_vector}
  \mathbf{F}=\begin{bmatrix}
    \sum_{j=1}^{m}(-1)^{1+j}A_{j}(\varphi(\mathbf{p}))M_{1,j}\\
    \vdots\\
    \sum_{j=1}^{m}(-1)^{m+j}A_{j}(\varphi(\mathbf{p}))M_{m,j}\\
  \end{bmatrix},
\end{equation}
and 
\begin{equation}
  \begin{aligned}
  D_{r,s}&=\{(z_{1},\ldots,z_{r-1},s,z_{r+1},\ldots,z_{m})|z_{i}\in(0,1)\},\\
  \tilde{z}_{r,s}&=(z_{1},\ldots,z_{r-1},s,z_{r+1},\ldots,z_{m}),\\
  \mathcal{D}_{r,s}&=\varphi(D_{r,s}),\\
  \end{aligned}
\end{equation}
by the divergence theorem on the simply connected region:
\begin{equation}
  \label{eq:GDT_Equiv_Form_2}
  \begin{aligned}
    I&=\oint_{\partial D^{m}}\mathbf{F}\cdot
    \mathbf{n}_{\partial D^{m}}\dif \mathbf{z}\\
    &=\sum_{r=1}^{m}\sum_{s=0}^{1}\int_{D_{r,s}}
    \mathbf{F}\cdot\mathbf{n}_{\partial D^{m}}\dif \mathbf{z}\\
    &=\sum_{r=1}^{m}\sum_{s=0}^{1}(-1)^{s+1}
    \int_{D^{m-1}}\sum_{j=1}^{m}(-1)^{r+j}A_{j}
    (\varphi(\tilde{z}_{r,s}))M_{r,j}\dif z_{1}
    \cdots\dif z_{r-1}\dif z_{r+1}\cdots\dif z_{m}\\
    &=\sum_{r=1}^{m}\sum_{s=0}^{1}\int_{\mathcal{D}_{r,s}}
    \mathbf{A}(\mathbf{x})\cdot\mathbf{n}_{\mathcal{S}}
    \dif \mathbf{x}\\
    &=\oint_{\mathcal{S}}\mathbf{A}\cdot
    \mathbf{n}_{\mathcal{S}}\dif \mathbf{x}.
  \end{aligned}
\end{equation}
The first step follows from the divergence theorem, 
and the fourth step from the definition of outward normal vector 
and $\mathbf{x}=\varphi(\mathbf{z})$. This completes the proof.
\end{proof}

\subsection{The proof of theorem \ref{thm:GeneralizedReynoldsTransportTheorem}}
\label{sec:pf_of_GRTT}
\begin{proof}
  We have
    \begin{equation}
    \begin{aligned}
    & \frac{\mathrm{d}}{\mathrm{d} t} 
    \left( \sum\limits_{n \in \mathbb{Z}\setminus 
    \left\{ 0 \right\}}^{}n\int\limits_{\mathcal{D}^{n}(t)}^{} 
    f (\mathbf{x},t)   \mathrm{d} \mathbf{x} \right)
    =  \frac{\mathrm{d}}{\mathrm{d} t} 
    \left( \int\limits_{D^{m}}^{} 
    f (\varphi (\mathbf{z},t),t) J_{\mathbf{z}} (\varphi) 
    \mathrm{d} \mathbf{z} \right)\\
    &=\int\limits_{D^{m}}^{} 
    \left(  \partial_{t}f+ \nabla_{\mathbf{z}} 
    f\cdot \partial_{t}\varphi+ f \nabla_{\mathbf{z}} 
    \cdot (\partial_{t}\varphi)\right) J_{\mathbf{z}} (\varphi) 
    \mathrm{d} \mathbf{z}\\
    &=\int\limits_{D^{m}}^{}   \partial_{t}f 
    J_{\mathbf{z}} (\varphi) \mathrm{d} \mathbf{z}+ 
    \int\limits_{D^{m}}^{} \nabla_{\mathbf{z}}
    \cdot(f\partial_{t}\varphi) J_{\mathbf{z}} (\varphi) 
    \mathrm{d} \mathbf{z}\\
    &=\sum_{n\in\mathbb{Z}\setminus\{0\}}n\int_{\mathcal{D}^{n}(t)}
    \partial_{t}f\dif\mathbf{x}+
    \int_{D^{m}}\sum_{j=1}^{m}\sum_{i=1}^{m}
    \pdfFrac{}{p_{i}}((-1)^{i+j}f\partial_{t}\varphi  M_{i,j})
    \dif\mathbf{p}\\
    &=\sum_{n\in\mathbb{Z}\setminus\{0\}}n\int_{\mathcal{D}^{n}(t)}
    \partial_{t}f\dif\mathbf{x}+\int_{\mathcal{S}(t)}f(\mathbf{y},t)
    \partial_{t}\varphi\cdot\mathbf{n}_{\mathcal{S}}\dif\mathbf{y}.
    \end{aligned}
    \end{equation}
    The first equality follows from the area formula, 
    the second equality follows from the Jacobi's formula, 
    and the divergence theorem and \eqref{eq:GDT_Equiv_form_1} 
    yield the fourth equality. 
    The last equality follows from $\mathbf{x}=\varphi(\mathbf{z})$, 
    $\mathcal{S}(t)=\varphi(\partial D^{m},t)$ 
    and \eqref{eq:GDT_Equiv_Form_2}.
\end{proof}
